# Supplementary material for: Parallel Stream Processing Against Workload Skewness and Variance
Source: arXiv:1610.05121 source file (2016-12-13)
Supplement: Supplementary file 1 [file appendix-lowboundexplanation.tex]

%%overview
\section{Low Bound Discussion}
{\color{red}
We omit the discussion of $ \theta_{min} $($ \theta_{min} = \max_{d\in\mathcal{D}}(\frac{\bar{L} -L(d) }{\bar{L}})$) in previous section because $\theta_{max}$ determines the bottleneck load. Moreover, the our algorithms make $\theta_{max} \geq \theta_{min} $.

Obviously, $ \theta_{max} = \theta_{min} $ when there only has two instances.
When $ N_{D} > 2 $, the biggest $ \theta_{max} $ is caused by each instance having the average load which will overload after loading $ c(k_{p})$.
For the same reason, the biggest $ \theta_{min} $ is caused by that instances having the same low load before loading the last $N_{D}-1$ bigger load keys. Assuming instance $d$ is the lowest instance after the last $N_{D}-1$ bigger keys being putted into other $(N_{D}-1)$ instance. Then the minimum load instance should be $ L(d) = \frac{\sum_{y \leq x-(N_{D}-1)}{c(y)}}{N_{D}} $, where $x$ is the position of the last bigger key.

In the worst case, $x = K$ and the last $N_{D}-1$ bigger load is $\frac{\overline{L}}{3}$, then the load of lowest instance is $\frac{N_{D} \cdot \overline{L} - (N_{D}-1) \cdot \frac{\overline{L}}{3}}{N_{D}}$ and $\theta_{min} = \frac{1}{3} \cdot (\frac{1}{N_{D}}-1)$. Therefore, $ \theta_{max} = \theta_{min}$. However, $K>x$ means that there are many keys with small granularity follow $x$. The \emph{Simple} algorithm will assign them to the lowest load instance, then $\theta_{max}$ will be unaffected while $\theta_{min}$ became smaller, so $\theta_{max} \geq \theta_{min}$.

{\color{blue}The phenomenon can be reflected by Fig.~\ref{fig:exp:skew}. Take $N_{D}=40$ in Fig.~\ref{fig:exp:parameterN} as an example. The up-bound can be calculated as $\max_{d\in\mathcal{D}}(\frac{L(d) - \bar{L}}{\bar{L}})$, where the average load $\bar{L}$ is defined as an unit load valued as 1.
And then $\theta_{max} \approx 0.8$ while low-bound $ \theta_{min} = \max_{d\in\mathcal{D}}(\frac{\bar{L} -L(d) }{\bar{L}}) \approx 0.2$. Furthermore, all lines in Fig.~\ref{fig:exp:parameterN} and Fig.~\ref{fig:exp:parameterK} verify our previous viewpoint that  $\theta_{max} \geq \theta_{min}$.
}}
