# Supplementary material for: Parallel Stream Processing Against Workload Skewness and Variance
Source: arXiv:1610.05121 source file (2016-12-13)
Supplement: Supplementary file 2 [file appendix-upboundproof_mylong.tex]

%%overview
\section{Proofs of Theorem 1 and Corollary 1}
{\color{red}
In order to derive theoretic results about the \emph{Mixed} algorithm, we first look at a more simplified key assignment algorithm, namely \emph{Simple} algorithm. Based on \emph{Simple}, we derive a group of theoretic analysis. Finally, we show how to establish the connection between \emph{Simple} and \emph{LLFD}, \emph{Min Table}, \emph{Min Mig} and \emph{Mixed} algorithms so that those derived results are applicable on our algorithms.

\textbf{Skeleton of proofs}

Step 1: Assuming ``Ideal'' load balance is achievable,  $k_p > 2 \cdot N_D$ and $c(k_p) \leq \frac{\bar{L}}{3}$.

Step 2: Assuming ``Ideal'' load balance is achievable,  for Simple Algorithm, $\theta_{\max} \leq \frac{1}{3}(1 - \frac{1}{N_D})$

Step 3: Given a general exptession of upbound and explain it.

Step 4: Prove the balance degree produced by \emph{LLFD}, \emph{Min Table}, \emph{Min Mig} and \emph{Mixed} is not worse than \emph{Simple}'s. 

\begin{algorithm}[t]
	%\small
	\caption{Simple Algorithm}
	\label{alg:simple}
	\begin{algorithmic}[1]
		\Require key candidate $\mathcal{C}$, task instances in $\mathcal{D}$
		\Ensure instances set $\mathcal{D}$ after loading keys
		\ForAll{$d$ in $\mathcal{D}$}
		\State add $k$ in instance $d$ to $\mathcal{C}$ 
		\State remove $k$ from instance $d$
		\EndFor
		\ForAll{$k$ in $\mathcal{C}$ in descending order of $c_{i-1}(k)$}
		\ForAll{$d$ in $\mathcal{D}$ in ascending order of $L_{i-1}(d)$}
		\State loading $k$ into instance $d$
		\EndFor
		\EndFor
		\State \Return instances set $\mathcal{D}$
	\end{algorithmic}
\end{algorithm}

As described in Alg.~\ref{alg:simple}, the \emph{Simple} algorithm works in the following way, at first, it disassociates and puts all the keys into the candidate set $\mathcal{C}$(lin 1 $\sim$ 3). Secondly it sorts these keys in the order of the computation cost $c(k)$. Finally it assigns each key to the instance with least total workload so far(lin 4 $\sim$ 6). 

\begin{definition}\label{def:cop}
	Assuming that \emph{Simple} algorithm is applied for key assignment. A key is defined as a ``problem maker'', denoted by $k_p$ with index $p$, if instances after assigned with this key according to \emph{Simple} algorithm, $\mathcal{D}$ will exist the largest overloaded in the result of loading.
\end{definition}

From Definition~\ref{def:cop}, we can infer that if there does not exist such $k_p$ in the process of loading keys into instance $\mathcal{D}$, no overloading on instance will happen during the key assignment process by the \emph{Simple} algorithm.

The following proposition states that the maximum degree of load imbalance by applying the \emph{Simple} algorithm is upper bounded.
In order to prove the upper bounded, we first introduce some lemmas.
\begin{lemma}\label{lem:lemma1}
	Given the instance set $\mathcal{D}$, key set $\mathcal{K}$ and the work load of each key $c(k)$, if there exists some approaches which can assign keys to instances achieving the perfect load balance, i.e, $\forall d_i, d_j\in\mathcal{D}, L(d_i) = L(d_j) = \bar{L} = \frac{1}{N_D}\sum_{k\in\mathcal{K}} c(k)$ and $\max_{k\in\mathcal{K}} c(k) < \bar{L}$, we have:
	\begin{equation}\label{equ:lemma}
	p > 2 \cdot N_D \ \ \textrm{and} \ \ c(k_p) \leq \dfrac{\bar{L}}{3}
	\end{equation}
	where key $k_p$ is the problem maker key and $p$ is the position of $k_p$ when the \emph{Simple} algorithm is applied.
	\end {lemma}
	\begin{proof}
		Assuming $ p = 2\cdot N_D$, there will be no overloaded instance. In such case, due to $\forall k \in \mathcal{K}, c(k)< \overline{L}$ and existing some approach which can assign keys to instances achieving the perfect load balance, then, each instance is associated with two keys.
		If $\exists d, L(d) > \overline{L}$, assume $L(d)$ is assigned with $ k_{i} $ and $ k_{j} $ where $ i \geq  j $(also means $c(k_{i}) \geq c(k_{j})$), then when assigning $ k_j$, $\nexists d' \in \mathcal{D}$, such that $d\neq d' \Rightarrow L(d') \leq L(d) $ according to \emph{Simple} algorithm preferentially assigns the biggest $c(k)$ to the lowest load instance;
		In other words $ \forall d' \in \mathcal{D} ,\ L(d') + c(k_j)>\overline{L}$, this is conflicts with the assumption that there exists some approach which can assign keys perfectly;
		If $ p < 2\cdot N_D $, then $\exists k \in \mathcal{K}, c(k) \geq \overline{L} $, this is contradicts with the assumption $\max_{k\in\mathcal{K}} c(k) < \bar{L}$.
		Therefore, it must have $p > 2\cdot N_D$.
		
		Secondly, assuming $c(k_p) > \frac{\bar{L}}{3}$, and $p = 2\cdot N_D+1$, then we have $ c(k_1)\geq c(k_2) \geq ... \geq c(k_{(2\cdot N_D)}) \geq c(k_{(2\cdot N_D+1)})>  \frac{\overline{L}}{3}$. In this case, no assignment algorithm is capable of achieving perfect load balance after loading those $2\cdot N_D+1$ keys, because any instance in $\mathcal{D}$ which had been assigned with the first $k_{(2\cdot N_D)}$ keys will become saturated for accepting the ($2\cdot N_D+1$)th key.
		Specifically, after the foregoing $(2\cdot N_D)$ keys been loaded into instance set $\mathcal{D}$, then $\forall d \in \mathcal{D}$, $L(d) > \frac{2}{3}\cdot\overline{L}$. Then, the $k_{(2\cdot N_D+1)}$ can not find a instance to sojourn under the un-overload constraint.
		However, the assumption in Lemma \ref{lem:lemma1} assumes that there exists some approach which can assign keys to instances achieving the perfect load balance,
		therefore, $c(k_p) \leq \frac{\bar{L}}{3}$
	\end{proof}

Now according to Definition~\ref{def:cop} and Lemma~\ref{lem:lemma1}, we can give the upbound of loading keys according to \emph{Simple} algorithm Theorem~\ref{theo:theorem1} as follows:

\begin{theorem}\label{theo:theorem1}
	Given the instance set $\mathcal{D}$, key set $\mathcal{K}$ and the work load of each key $c(k)$, if there exists some approaches which can assign keys to instances achieving the perfect load balance, i.e, $\forall d_i, d_j\in\mathcal{D}, L(d_i) = L(d_j) = \bar{L} = \frac{1}{N_D}\sum_{k\in\mathcal{K}} c(k)$, then by applying the Simple algorithm for the assignment, we have the upper bound of imbalance tolerance as follows:
	\begin{equation}\label{equ:idealtheta}
	\theta_{max} \leq \dfrac{1}{3} \cdot (1-\dfrac{1}{N_D}) + 1,
	\end{equation}
	where $\theta_{max} = \max_{d\in\mathcal{D}}(\frac{L(d) - \bar{L}}{\bar{L}})$
\end{theorem}

\begin{proof}
	According to Lemma~\ref{lem:lemma1}, $p > 2 \cdot N_D \ \ \textrm{and} \ \ c(k_p) \leq \frac{\bar{L}}{3}$, it is obviously that the load of "problem maker" key $c(k_{p}) = \frac{\bar{L}}{3}$ will incur the largest overload instance.
	We first assume the "problem maker" key is lie in the $(2\cdot N_{D}+1)$th position.
	Then, before the $(k_{(2\cdot N_{D})+1})$th key being loaded into the instance set $\mathcal{D}$, there are $(k_{(2\cdot N_{D})})$ largest keys which had been put into $\mathcal{D}$.
	According to \emph{Simple} algorithm, if the load of $(k_{(2\cdot N_{D})})$ largest keys in $\mathcal{D}$ are even, the overload is largest after loading the  $(k_{(2\cdot N_{D})+1})$th key.
	The largest total load of the first $(k_{(2\cdot N_{D})})$ keys should be $N_D \cdot \overline{L} - \frac{\overline{L}}{3}$.
	Then, the average load of instances before $k_p$ assigned is $\frac{N_D \cdot \overline{L} - \frac{\overline{L}}{3}}{N_D}$. After $k_p$ is assigned, the max load($L_{\max}$) on instances can be expressed as:
	\begin{equation}\label{equ:ML}
	L_{\max} = \frac{N_D \cdot \overline{L} - \frac{\overline{L}}{3}}{N_D} + \dfrac{\overline{L}}{3} 
	\end{equation}
	Based on $\theta_{max} = \frac{L_{\max} - \bar{L}}{\bar{L}}$ and  Equation \ref{equ:ML}, the upper bound of $\theta_{max}$ can be expressed by Equation.~\ref{equ:idealtheta}.
	
	Secondly, if the "problem maker" key $k_{p}$ does not locate at the $(k_{(2\cdot N_{D}+1)})$th position, then $p > k_{(2\cdot N_{D})+1}$ according to Lemma~\ref{lem:lemma1}. Then the max load can be expressed as $ \frac{\sum_{i \in [1,p-1]}c(k_{i})}{N_D} + c(k_{p})$.
	In any case, however, $\sum_{i \in [1,p-1]}c(k_{i}) \leq N_D \cdot \overline{L} - c(k_{p})$ is true. 
	Then we have \begin{equation}\label{equ:unequal} \frac{\sum_{i \in [1,p-1]}c(k_{i})}{N_D} + c(k_{p}) \leq \frac{N_D \cdot \overline{L} - c(k_{p})}{N_D} + c(k_{p})\end{equation}
	Due to $N_D \geq 1$, then $c(k_{p})$ is proportional to the right part of Equation.~\ref{equ:unequal}. Furthermore, $c(k_p) \leq \frac{\bar{L}}{3}$ according to Lemma~\ref{lem:lemma1}, then the maximum amount of overload in the right part of Equation.~\ref{equ:unequal} is $c(k_{p}) = \frac{\overline{L}}{3}$. In this case, the right part of Equation.~\ref{equ:unequal} is equal to Equation \ref{equ:ML}.
	And then, Theorem~\ref{theo:theorem1} is proved.
\end{proof}

The next Lemma is a direct extension of Theorem~\ref{theo:theorem1}.
\begin{lemma}\label{lem:lemmageneral}
Given the instance set $\mathcal{D}$, key set $\mathcal{K}$ and the work load of each key $c(k)$, if there exists some approach which can assign keys to instances achieving the perfect load balance, i.e, $\forall d_i, d_j\in\mathcal{D}, L(d_i) = L(d_j) = \bar{L} = \frac{1}{N_D}\sum_{k\in\mathcal{K}} c(k)$, then by applying the \emph{Simple} algorithm for the assignment, we have:
\begin{equation}\label{equ:morekeytheta}
\theta_{max} \leq \dfrac{c(k_p) - \frac{c(k_p)+ \sum_{j=p+1}^{K}c(k_j)}{N_D}}{\bar{L}}, \end{equation}
\end {lemma}
where $\theta_{max} = \max_{d\in\mathcal{D}}(\frac{L(d) - \bar{L}}{\bar{L}})$
\begin{proof}
As described in the proof of Theorem~\ref{theo:theorem1}, before assiging $c(k_p)$, there was $ N_D \cdot \bar{L} - c(k_p) - \sum_{j=p+1}^{K}c(k_j)$ load had been assigned into $N_D$ instances. And then, the average load of instances is $\frac{N_D \cdot \bar{L} - c(k_p) - \sum_{j= p+1}^{K} c(k_j)}{N_D}$ and the max load instance ($L_{\max}$) after assign $k_p$ into instance can expressed as 
$\frac{N_D \cdot \bar{L} - c(k_p) - \sum_{j=p+1}^{K} c(k_j)}{N_D}$ $+ c(k_p)$.
Based on this expression and $\theta_{max} = \frac{L_{\max} - \bar{L}}{\bar{L}}$, the upper bound of $\theta_{max}$ can be expressed as Eq.~(\ref{equ:morekeytheta})
\end{proof}

Usually, the number of keys is more than the number of instances ($K
\gg |\mathcal{D}|$) and the accumulative load for the tails in skewed
data distribution is significant.
In other words, if the load of "problem maker" $c(k)$ is larger, the part of $\frac{c(k_p)+ \sum_{j=p+1}^{K}c(k_j)}{N_D}$ in Eq.~(\ref{equ:morekeytheta}) is much larger for the long tail distribution.
Therefore, we believe that the \emph{Simple} algorithm can produce a well-balanced adjustment.

\eat{Now, we use Lemma ~\ref{lem:lemmageneral} to verify the balance assignment effect of \emph{Simple} algorithm for a common skew distribution \emph{Zipf distribution}. Namely, assuming ``Ideal'' load balance is achievable and the $c(k)$ of keys follows a \emph{Zipf distribution},  for \emph{Simple} algorithm, $\theta_{\max} \rightarrow 0$. 
Specifically, assuming the load of keys follows the \emph{Zipf distribution} and the skewed degree $z=1$, after applying the \emph{Simple} algorithm, the maximum degree of load imbalance among instances in $\mathcal{D}$ achieves zero.
The specific explanation as follows:
We assume the unit load is 1, then the load set is $ G = \lbrace c(k_{x})\vert 1 \leq x \leq K \rbrace = \lbrace K,\frac{K}{2},...,\frac{K}{K-1},1 \rbrace $.
According to Fig.~\ref{fig:exp:parameterN} in Sec.~\ref{sec:evaluations} that the skewness of instance is proportional to the number of instance $|\mathcal{D}|$, we find the maximal number of $|\mathcal{D}|$ as the candidate instance set.
Due to $c(k) \leq \bar{L}$ and then the maximum number of instance $|\mathcal{D}|$ is  $\frac{\sum_{x=1}^{K}\frac{K}{x}}{K}= ln(K)+\gamma$\footnote{$\gamma$ is Euler-Mascheroni constant $\gamma \approx 0.5772156649$}. Now we assume exist "problem maker" $c(k_p)$ in $G$ and then use Equation \ref{equ:morekeytheta}, $\theta_{max}$ can be expressed as
\[\frac{\frac{K}{cop}-\frac{(ln(K-cop)+r) \cdot K}{ln(K)+r}}{K} < 0.\] 
Therefore,we believe that there is no $cop$ in zipf distribution and it can be perfect partition use the Simple algorithm.}

\begin{theorem}\label{theo:theorem3}
The balance degree produced by \emph{LLFD}, \emph{Min Table}, \emph{Min Mig} and \emph{Mixed} is not worse than \emph{Simple}'s.
\end {theorem}

We only take \emph{Mixed} algorithm as an example to prove Theorem ~\ref{theo:theorem3} and the proof for others algorithm is similar.
\begin{proof}
For \emph{Mixed} algorithm, Theorem ~\ref{theo:theorem3} means that the balance status generated by the \emph{Mixed} represented by $\theta_{Mix}$ is not worse than the balance status $\theta_{Sim}$ produced by the \emph{Simple} algorithm.
Supposing $\theta_{Mix} > \theta_{Sim}$, and now we take $\theta_{Sim}$ as the upper bound of imbalance tolerance $\theta_{max}$, then the \emph{Mixed} algorithm produces overload instance(s), in other words, $\exists c(k_p)$ in \emph{Mixed}'s migration process incurs that the overload is bigger than $\theta_{Sim}$. Because the \emph{Mixed} tries all instances to put $c(k_{p})$ to eliminate overload as shown in Algorithm~\ref{alg:Mixed}, then $\theta_{Mix} > \theta_{Sim}$ means that $\forall d$, $d \in \mathcal{D}$, $c(k_{p})+ L(d) - \sum_{k' \in \lbrace k'' | c(k'') < c(cop) \rbrace}{c(k')}$ is larger than upbound. In this case, \emph{Simple} algorithm also can not assign $c(k_{p})$ to $\mathcal{D}$ without exceeds the upbound. Then the balance degree produced by \emph{Mixed} is not worse than \emph{Simple}'s.
\end{proof}
}
